# Supplementary material for: Design and Evaluation of Scalable Representations of Communication in Gantt Charts for Large-scale Execution Traces
Source: arXiv:2107.00065 source file (2021-08-17)
Supplement: Supplementary file 1 [file Scalable_Designs_Expert_Feedback_Prompt.pdf]

# Communication Designs Primer


## Abstract

Logical time is used in visualizations like Ravel to reveal communication patterns. However, this only works at small scales (e.g., 64 processors or less). We seek to design representations to use at larger scales that trade off exactness for more easily communicating the patterns. This document describes the patterns we chose and our proposed representations.


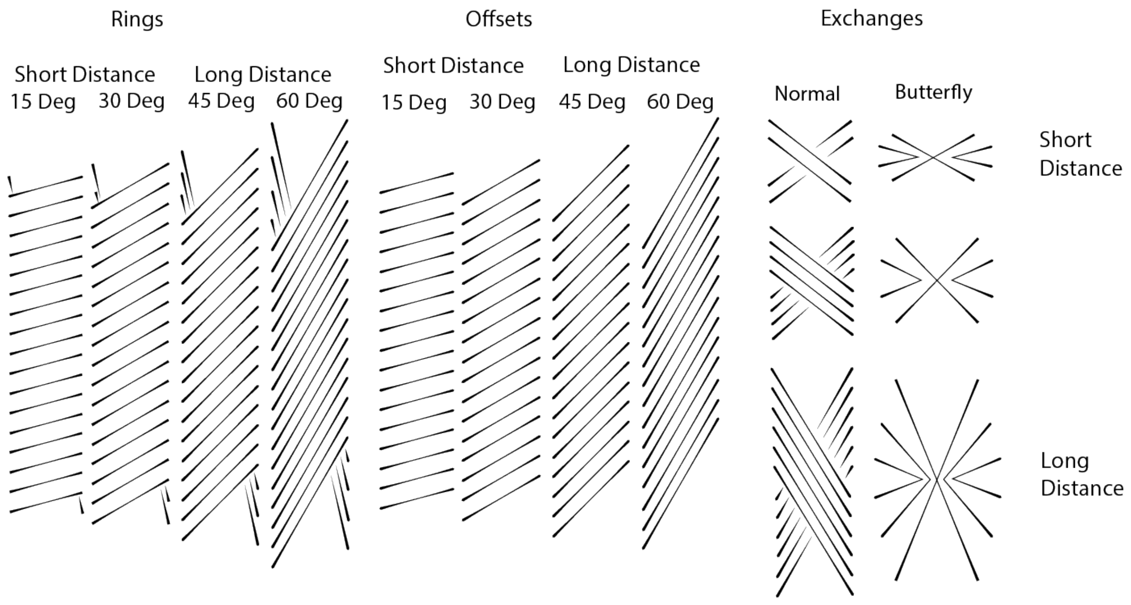


Figure 1: Our designs for large scale representations of communication patterns in Ravel Gantt charts

## The Designs

In Figure 2, we see an example of a Gantt chart visualizing the communication between processes running on 64 nodes. This is a rather clean example of how communication patterns occur visually in Gantt charts. By rendering the physical lines in 1-to-1 detail, looking at this chart can be borderline headache-inducing and make scanning for information difficult. Furthermore, distinguishing between particular patterns like "exchanges" and "rings" in the center portion can be difficult.

To solve these problems and more, we have developed a collection of visual symbols which summarize information about these patterns. We hope that it will aid when looking at these charts in cases where these communications are reduced to a hairball of overlapping lines. The basic structure of these designs can be seen in Fig. 1.

These symbols aim to make two characteristics of underlying patterns clear at a glance:

1. The underlying pattern itself (ring, offset, or exchange)

2. The relative distance between senders and receivers (shown with the steepness of angles)

We have modified Figure 2 to show more concretely how these designs may help at a glance assessments of HPC communication. (Figure 3)

1. Several columns which share similar characteristics are grouped into a single, large symbol

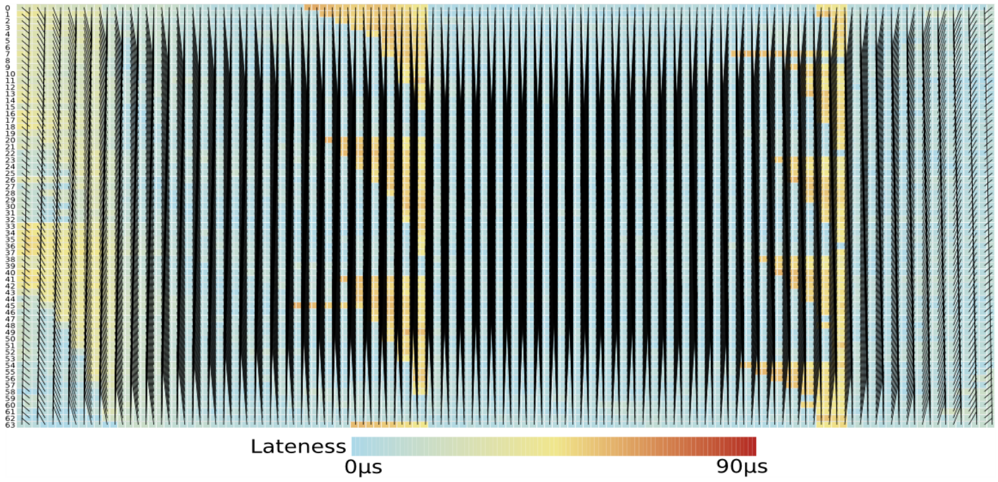


Figure 2: A Ravel chart showing communication between 64 nodes.

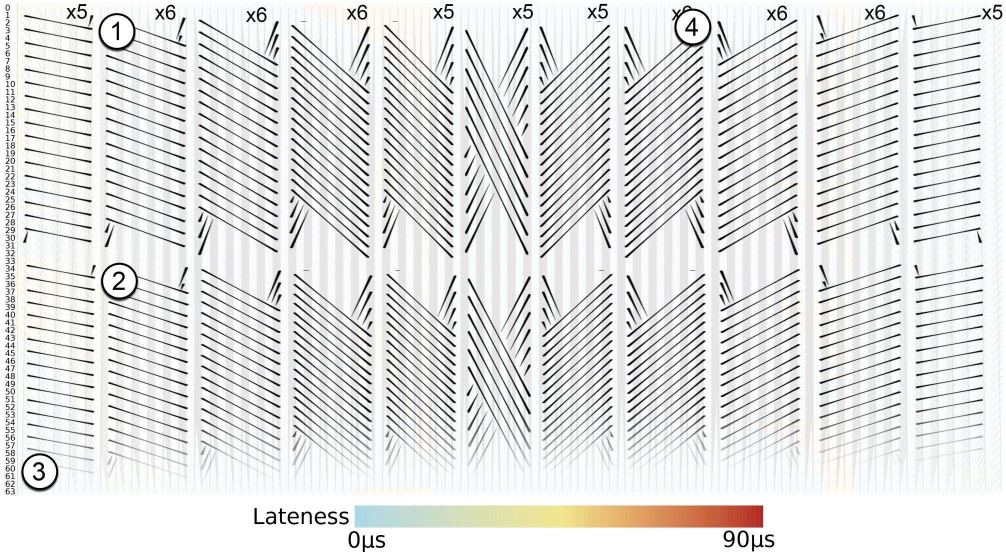


Figure 3: A mock-up of a Ravel chart which aggregates the hard to see large scale communications data into a few symbols. The x numbers at the top indicate that these primitives encompass that number of underlying columns of patterns.

2. If this patterns repeats, possibly beyond the 64 nodes shown here, we show that by doubling up the pattern

3. If part or all of a pattern continues past the view area, it is shown with an opacity gradient

4. The orientation of the calls – e.g. whether the majority of calls are being sent to "higher" nodes or "lower" nodes – is encoded by flipping our base symbols horizontally

Figure 5 shows an example of what Figure 4 would look like with our designs:

1. In this column we see that there are repeating groups of butterfly exchange patterns.

2. Overlapping, different patterns are rendered next to each other.

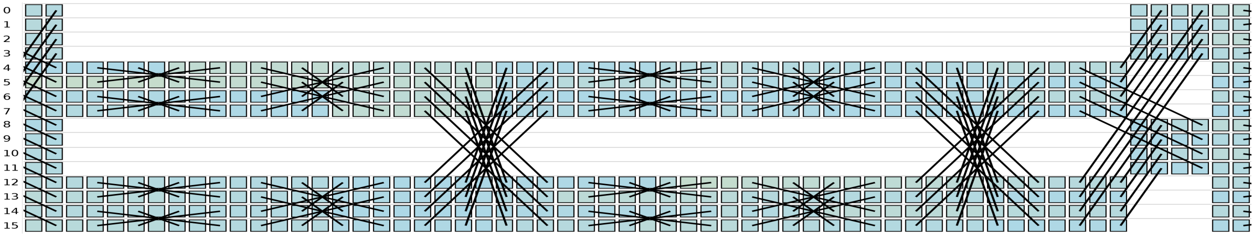


Figure 4: A Ravel chart showing execution of a parallel MG algorithm.

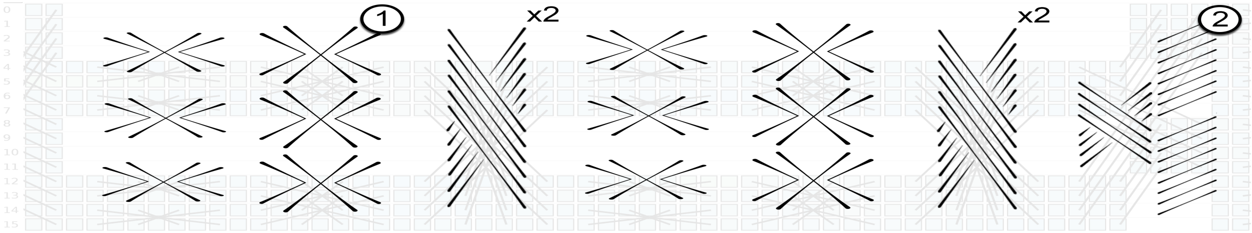


Figure 5: A mock-up showing additional information our designs provide at a glance.

## Questions

Hopefully this has given you enough information about our proposed designs that you may be able to answer the following questions for us.

1. Would this be helpful? If so, how?
2. Do you have any suggestions or concerns?
