# Supplementary material for: Design and Evaluation of Scalable Representations of Communication in Gantt Charts for Large-scale Execution Traces
Source: arXiv:2107.00065 source file (2021-08-17)
Supplement: Supplementary file 2 [file pilots.tex]

\section{Study Pilots} 

\subsection{Original Pilot}

\subsection{Drawing Pilot}
% study purpose
To follow up from our prior experiment, we wanted to explore exactly what a controlled experiment might look like to help us understand how people might perceive patterns of communication lines. Thinking that there may be merit in allowing users to extrapolate patterns or themselves from an image of partially rendered communication lines, we created a pen and paper experiment focused around this idea. This study was executed on a cross section of attendee’s to Hack Arizona – recruited with stuffed animal toys – totaling 15 respondents.

For the study itself, we supplied participants with a packet of five questions with each question containing either a partial or full rendering of communication lines over two boxes simulating a Gantt chart. For each question, next to the image, we printed an empty grid of boxes, two columns wide and 12 rows long. In both the partial and full cases, we asked users to draw a pattern over the 24 boxes equivalent to the pattern shown on the associated ``chart." In addition to drawing lines, respondents were provided with crayons and asked to color in boxes to match the pattern of boxes on the left. Finally, per question, participants were also asked to rate their perceived difficulty of that question and how confident they were in their correctness. 

Before being exposed to the main packet of questions, individuals were introduced to the experiment with two basic questions of the same type as the rest of the experiment in a tutorial phase. During this phase, subjects were supervised by an experiment conductor and encouraged to ask questions as they went through this mini packet. After the tutorial concluded, participants could no longer ask questions or seek assistance as they went through the main packet of questions.

Responses were evaluated with a semi-subjective grading process where correctness was quantified on a 4 point scale. After this quantification it was determined that nearly half of all responses had to be thrown out due to fundamentally incorrect responses. In most of these cases, participants would replicate patterns very literally, disregarding the idea that one line connects two boxes and instead multiple lines spanning two boxes. These errors were like due to ambiguities in the question prompt and insufficient materialization. 

Concerning the second study, unfortunately, as so much data had to be thrown out there was not enough remaining to make conclusions about how our independent variables of pattern and partial/full rendering type affected our dependant variable of response accuracy. Regardless, we do conclude that at this stage in our experiment design process, it would not be worth implementing this type of free-form experiment into a digital platform due to our observed difficulty of getting participants to understand the intent of the experiment. 

\subsection{3rd Pilot}

\subsection{4th Pilot}
